# Supplementary material for: Zero-shot Transfer Learning of Driving Policy via Socially Adversarial Traffic Flow
Source: arXiv:2304.12821 source file (2023-04-25)
Supplement: Supplementary file 1 [file 6-appendix.tex]

\clearpage

\section{Appendix}
\subsection{Implementation Details}

{\bf{Intelligent Driver Model (IDM)}}. IDM is given by \Eqref{eq:IDM1} and \Eqref{eq:IDM2}. The model describes the acceleration $\dot{v}_{back}$ of the back agent, as a function of the agent's velocity $v_{back}$, the reference velocity $v_0$, the difference between the agent velocity and the velocity of the agent in front $\Delta v=v_{back}-v_{front}$, and the following distance $\varphi=s_{front}+L_{length,front}-s_{back}$. Here, $s_{front}$ is the position of the front agent, $s_{back}$ denotes the position of the back agent, and $L_{length, front}$ denotes the length of the front agent. The physical interpretation of the parameters are the minimum following time, $T$, the minimum following gap, $s_0$, the maximum acceleration, $a$, the minimum following gap, $s_0$, the maximum acceleration, $a$, and the comfortable braking deceleration, b.
\begin{align}
    &\dot{v}_{back}=a\left[1-\left(\frac{v_{back}}{v_{0}}\right)^{\delta}-\left(\frac{\phi\left(v_{back}, \Delta v\right)}{\varphi}\right)^{2}\right]    \label{eq:IDM1}\\
    &\phi\left(v_{back}, \Delta v\right)=s_{0}+v_{back} T+\frac{v_{back} \Delta v}{2 \sqrt{a b}}      \label{eq:IDM2}
\end{align}

{\bf{Policy learning parameters.}} For Independent Policy Learning (IPL) and single-agent reinforcement learning algorithms, we utilize Soft-Actor-Critic (SAC) \cite{haarnoja2018soft} and Adam optimizer \cite{kingma2015adam}. Detailed parameters are shown in \Tabref{table:sac-param}.

\subsection{Results on Our Coordinated Traffic Flow} \label{appendix:section-flow}

\subsection{Results on Zero-shot Transfer} \label{appendix:section-transfer}

More results are shown in \Tabref{appendix-table:ood-performance-intersection}, \Tabref{appendix-table:ood-performance-bottleneck} \Tabref{appendix-table:ood-performance-merge}, \Tabref{appendix-table:ood-performance-roundabout}.

% \subsection{Additional Results} \label{appendix:additional-results}

% {\color{blue} The comparison of training efficiency between CoPO and SocialComm (Ours) is shown in \Figref{figure:train-curve}.}

% {\color{blue} The impact of varying the number of agents in each scenario is shown in \Figref{figure:flow-vary-number}.}

\begin{table*}[ht]
\centering
\caption{{\bf {Parameters of IDM.}}}
\label{table:idm-param-1}
\begin{tabular}{p{4cm}   c c c c l  c c c c}
    \toprule
    Parameter & Value     \\ 
    \midrule 
    Desired speed $v_0$ &   6 $m/s$  \\
    Time gap $T$                &  1.0 $s$        \\
    Minimum gap $s_0$             & 2 $m$                   \\
    Acceleration exponent $\delta$     & 4            \\
    Acceleration $a$            &  5.0 $m/s^2$ \\
    Comfortable deceleration $b$  &  5.0 $m/s^2$  \\ 

    \toprule
\end{tabular}
\end{table*}

\begin{table}[ht]

\centering
\caption{{\bf {Hyperparameters of SAC.}}}
\label{appendix-table:sac-param}
\vspace{1mm}
\begin{tabular}{l l }
\toprule
{Parameter} & Value\\
\midrule
    optimizer &Adam\\
    actor learning rate & $1 \cdot 10^{-4}$\\
    critic learning rate & $5 \cdot 10^{-4}$\\
    tune learning rate & $1 \cdot 10^{-4}$\\
    discount ($\gamma$) &  0.9\\
    batch size & 128\\
    replay buffer size & $10^6$\\
    nonlinearity & ReLU\\
    target smoothing coefficient ($\tau$)& 0.005\\
    target update interval & 1\\
    gradient steps & 1\\
\bottomrule
\end{tabular}
\end{table}

\begin{table*}[t]
\centering
\caption{{\bf {Quantitative performance of traffic flows.}} The table reports the percentage of different metrics in \texttt{intersection}, \texttt{bottleneck}, \texttt{merge}, and \texttt{roundabout}. A ``$^\dagger$" indicates the proposed traffic flow.}
\resizebox{\textwidth}{!}{
\begin{tabular}{b{2.6cm}<{\centering}   c c c c c c  }
    \toprule
    \multirow{2}{*}[-0.5em]{\makecell[c]{\vspace{0.1cm}Traffic Flows}} & \multicolumn{6}{c}{\texttt{Intersection}}  \\
    \cline{2-7}  \vspace{-3mm}\\ 
    & Success ($\uparrow$) & Collision ($\downarrow$) & Off Road ($\downarrow$) & Off Route ($\downarrow$) & Wrong Lane ($\downarrow$) & Efficiency ($\uparrow$)   \\
    \cline{1-7}  \vspace{-2mm}\\ 
    \rowcolor{priormethod} {IDM}                     & 70.4 $\pm$ 0.0  & 29.6 $\pm$ 0.0  & \textbf{0.0 $\pm$ 0.0}  & \textbf{0.0 $\pm$ 0.0}  & \textbf{0.0 $\pm$ 0.0} &  42.1 $\pm$ 0.0  \\
    \rowcolor{priormethod} {FLOW}                    & 79.6 $\pm$ 0.5  & 15.9 $\pm$ 0.6  & 2.0 $\pm$ 0.2  & 1.2 $\pm$ 0.1  & \textbf{0.0 $\pm$ 0.0}  & 47.4 $\pm$ 0.2   \\
    \rowcolor{priormethod} {CoPO}             & 79.6 $\pm$ 0.3  & 17.6 $\pm$ 0.4  & 1.3 $\pm$ 0.1  & 1.4 $\pm$ 0.1  & 0.1 $\pm$ 0.1  & 46.8 $\pm$ 0.1    \\
    \rowcolor{priormethod} {FailMaker}             & 45.3 $\pm$ 0.3  & 52.5 $\pm$ 0.3  & \textbf{0.0 $\pm$ 0.0}  & \textbf{0.0 $\pm$ 0.0}  & \textbf{0.0 $\pm$ 0.0}  & 28.7 $\pm$ 0.1   \\
    \rowcolor{priormethod} {SocialComm}$^\dagger$    & \textbf{86.9 $\pm$ 0.5}   & \textbf{9.0 $\pm$ 0.4}  & 2.8 $\pm$ 0.1  & 1.2 $\pm$ 0.1  & 0.2 $\pm$ 0.1 & \textbf{51.0 $\pm$ 0.2}  \\
    \bottomrule
\end{tabular}
}

\resizebox{\textwidth}{!}{
\begin{tabular}{b{2.6cm}<{\centering}   c c c c c c  }
    \multirow{2}{*}[-0.5em]{\makecell[c]{\vspace{0.1cm}Traffic Flows}} & \multicolumn{6}{c}{\texttt{Bottleneck}}  \\
    \cline{2-7}  \vspace{-3mm}\\ 
    & Success ($\uparrow$) & Collision ($\downarrow$) & Off Road ($\downarrow$) & Off Route ($\downarrow$) & Wrong Lane ($\downarrow$) & Efficiency ($\uparrow$)   \\
    \cline{1-7}  \vspace{-2mm}\\ 
    \rowcolor{priormethod} {IDM}                       & 67.0 $\pm$ 0.0   & 33.0 $\pm$ 0.0   & \textbf{0.0 $\pm$ 0.0}  & \textbf{0.0 $\pm$ 0.0}   & \textbf{0.0 $\pm$ 0.0}   & 49.1 $\pm$ 0.0 \\
    \rowcolor{priormethod} {FLOW}                     & 76.2 $\pm$ 0.5   & 9.8 $\pm$ 0.4   & 14.3 $\pm$ 0.6   & \textbf{0.0 $\pm$ 0.0}   & \textbf{0.0 $\pm$ 0.0}   & 75.1 $\pm$ 0.3 \\
    \rowcolor{priormethod} {CoPO}               & 80.3 $\pm$ 0.6   & \textbf{9.3 $\pm$ 0.7}   & 11.4 $\pm$ 0.4   & \textbf{0.0 $\pm$ 0.0}   & \textbf{0.0 $\pm$ 0.0}  & 74.5 $\pm$ 0.3  \\
    \rowcolor{priormethod} {FailMaker}             & 21.3 $\pm$ 0.2  & 78.6 $\pm$ 0.1  & 0.1 $\pm$ 0.0  & \textbf{0.0 $\pm$ 0.0}  & \textbf{0.0 $\pm$ 0.0}  & 29.0 $\pm$ 0.2 \\
    \rowcolor{priormethod} {SocialComm}$^\dagger$     &\textbf{83.4 $\pm$ 0.4}   & 9.4 $\pm$ 0.3   & 7.3 $\pm$ 0.3   & \textbf{0.0 $\pm$ 0.0}   & \textbf{0.0 $\pm$ 0.0}  & \textbf{76.4 $\pm$ 0.1}  \\
    \bottomrule
\end{tabular}
}

\resizebox{\textwidth}{!}{
\begin{tabular}{b{2.6cm}<{\centering}   c c c c c c  }
    \multirow{2}{*}[-0.5em]{\makecell[c]{\vspace{0.1cm}Traffic Flows}} & \multicolumn{6}{c}{\texttt{Merge}}  \\
    \cline{2-7}  \vspace{-3mm}\\ 
    & Success ($\uparrow$) & Collision ($\downarrow$) & Off Road ($\downarrow$) & Off Route ($\downarrow$) & Wrong Lane ($\downarrow$) & Efficiency ($\uparrow$)   \\
    \cline{1-7}  \vspace{-2mm}\\ 
    \rowcolor{priormethod} {IDM}                     & 60.0 $\pm$ 0.0   & 40.0 $\pm$ 0.0   & \textbf{0.0 $\pm$ 0.0}   & \textbf{0.0 $\pm$ 0.0}   & \textbf{0.0 $\pm$ 0.0}   & 46.9 $\pm$ 0.0    \\
    \rowcolor{priormethod} {FLOW}                    & 66.2 $\pm$ 0.4   & 25.4 $\pm$ 0.5   & 8.5 $\pm$ 0.2   & \textbf{0.0 $\pm$ 0.0}   & \textbf{0.0 $\pm$ 0.0}  &  55.1 $\pm$ 0.2  \\
    \rowcolor{priormethod} {CoPO}             & 69.3 $\pm$ 0.5   & 26.9 $\pm$ 0.6   & 3.8 $\pm$ 0.3   & \textbf{0.0 $\pm$ 0.0}   & \textbf{0.0 $\pm$ 0.0}   & 54.9 $\pm$ 0.2     \\
    \rowcolor{priormethod} {FailMaker}             & 16.0 $\pm$ 0.2  & 80.9 $\pm$ 0.2  & 3.4 $\pm$ 0.2  & \textbf{0.0 $\pm$ 0.0}  & \textbf{0.0 $\pm$ 0.0}  & 16.2 $\pm$ 0.1  \\
    \rowcolor{priormethod} {SocialComm}$^\dagger$    & \textbf{83.1 $\pm$ 0.5}   & \textbf{16.2 $\pm$ 0.5}   & 0.6 $\pm$ 0.1   & 0.2 $\pm$ 0.1   & \textbf{0.0 $\pm$ 0.0}  & \textbf{60.0 $\pm$ 0.2}   \\
    \bottomrule
\end{tabular}
}

\resizebox{\textwidth}{!}{
\begin{tabular}{b{2.6cm}<{\centering}   c c c c c c  }
    \multirow{2}{*}[-0.5em]{\makecell[c]{\vspace{0.1cm}Traffic Flows}} & \multicolumn{6}{c}{\texttt{Roundabout}}  \\
    \cline{2-7}  \vspace{-3mm}\\ 
    & Success ($\uparrow$) & Collision ($\downarrow$) & Off Road ($\downarrow$) & Off Route ($\downarrow$) & Wrong Lane ($\downarrow$) & Efficiency ($\uparrow$)   \\
    \cline{1-7}  \vspace{-2mm}\\ 
    \rowcolor{priormethod} {IDM}                      & 73.6 $\pm$ 0.0   & 26.4 $\pm$ 0.0   & \textbf{0.0 $\pm$ 0.0}   & \textbf{0.0 $\pm$ 0.0}   & \textbf{0.0 $\pm$ 0.0}   & 38.1 $\pm$ 0.0  \\
    \rowcolor{priormethod} {FLOW}                     & 72.7 $\pm$ 0.6   & 22.4 $\pm$ 0.4   & 4.8 $\pm$ 0.2   & \textbf{0.0 $\pm$ 0.0}   & 0.1 $\pm$ 0.1   & 39.2 $\pm$ 0.1  \\
    \rowcolor{priormethod} {CoPO}               & 81.2 $\pm$ 0.6   & 14.3 $\pm$ 0.5   & 4.0 $\pm$ 0.2   & \textbf{0.0 $\pm$ 0.0}   & 0.5 $\pm$ 0.1   & 39.0 $\pm$ 0.1   \\
    \rowcolor{priormethod} {FailMaker}               & 21.3 $\pm$ 0.3  & 77.6 $\pm$ 0.3  & 0.5 $\pm$ 0.0  & \textbf{0.0 $\pm$ 0.0}  & 0.6 $\pm$ 0.1  & 15.7 $\pm$ 0.1 \\
    \rowcolor{priormethod} {SocialComm}$^\dagger$       & \textbf{84.6 $\pm$ 0.5}   & \textbf{11.5 $\pm$ 0.3}   & 3.6 $\pm$ 0.3   & 0.1 $\pm$ 0.0   & 0.5 $\pm$ 0.1   & \textbf{42.2 $\pm$ 0.1} \\
    \bottomrule
\end{tabular}
}

\label{appendix-table:traffic-simulation}
\end{table*}

\begin{table*}[htb]
\centering
\caption{{\bf {Zero-shot transfer performance in \texttt{intersection}.}} Each subtable stores results of different driving policies in the same traffic flow. A ``$^\dagger$" indicates the proposed method.}
\label{appendix-table:ood-performance-intersection}
 % default is 1.0
\resizebox{\textwidth}{!}{
\begin{tabular}{b{3.5cm}<{\centering}   c c c c c c  }
    \toprule
    \multirow{2}{*}[-0.5em]{\makecell[c]{\vspace{0.1cm}Evaluate in \\ FailMaker}} & \multicolumn{6}{c}{\texttt{Intersection}}  \\
    \cline{2-7}  \vspace{-3mm}\\ 
    & Success ($\uparrow$) & Collision ($\downarrow$) & Off Road ($\downarrow$) & Off Route ($\downarrow$) & Wrong Lane ($\downarrow$) & Efficiency ($\uparrow$)   \\
    \cline{1-7}  \vspace{-2mm}\\ 
    \rowcolor{ourmethod} {RARL/FailMaker}        & 26.5  & 11.5  & 17.5  & 14.5  & 0.0  & 25.9     \\
    \rowcolor{priormethod} {VRL/IDM}            & \textbf{55.0}  & \textbf{22.5}  & 22.0  & \textbf{0.0}  & 0.5  & \textbf{37.3}   \\
    \rowcolor{priormethod} {VRL/FLOW}           & 52.0  & 37.0  & 12.0  & \textbf{0.0}  & \textbf{0.0}  & 36.0  \\
    \rowcolor{priormethod} {VRL/CoPO}            & 51.0  & 43.5  & \textbf{4.0}  & 1.0  & 0.5  & 34.7   \\
    \rowcolor{priormethod} {VRL/SocialComm}    & 51.5  & 33.0  & 16.5  & 1.5  & \textbf{0.0}  & 36.5   \\
    \rowcolor{priormethod} {M-RARL/SocialComm}$^\dagger$     & 51.0  & 40.5  & 8.0  & \textbf{0.0}  & \textbf{0.0}  & 35.9   \\
    % \rowcolor{priormethod} {M-RARL/SocialComm}$^\dagger$     & 53.5  & 36.0  & 10.5  & 0.0  & 0.0  & 36.6  \\
    \bottomrule
\end{tabular}}
\resizebox{\textwidth}{!}{
\begin{tabular}{b{3.5cm}<{\centering}   c c c c c c  }
    \multirow{2}{*}[-0.5em]{\makecell[c]{\vspace{0.1cm}Evaluate in \\ IDM}} & \multicolumn{6}{c}{\texttt{Intersection}}  \\
    \cline{2-7}  \vspace{-3mm}\\ 
    & Success ($\uparrow$) & Collision ($\downarrow$) & Off Road ($\downarrow$) & Off Route ($\downarrow$) & Wrong Lane ($\downarrow$) & Efficiency ($\uparrow$)   \\
    \cline{1-7}  \vspace{-2mm}\\ 
    \rowcolor{priormethod} {RARL/FailMaker}                & 22.5  & \textbf{20.5}  & 19.5  & 11.0  & \textbf{0.0}  & 25.2    \\
    \rowcolor{ourmethod} {VRL/IDM}            & 79.5  & 6.0 & 2.0 & 0.0 & 0.0&  47.1  \\
    \rowcolor{priormethod} {VRL/FLOW}           & 67.0 & 30.5 & \textbf{0.5} & 0.5 & 0.5&  39.5  \\
    \rowcolor{priormethod} {VRL/CoPO}            & 69.0 & 27.0 & \textbf{0.5} & \textbf{0.0} & \textbf{0.0} & \textbf{43.0}  \\
    \rowcolor{priormethod} {VRL/SocialComm}    & 69.0 & 28.5 & 3.5 & 2.0 & \textbf{0.0}& 40.8 \\
    \rowcolor{priormethod} {M-RARL/SocialComm}$^\dagger$     & \textbf{71.5} & 21.5 & 6.0 & 1.0 & \textbf{0.0} &  42.1  \\
    % \rowcolor{priormethod} {M-RARL/SocialComm}$^\dagger$     & 74.0  & 24.0  & 0.0  & 0.0  & 0.0  & 43.8  \\
    \bottomrule
\end{tabular}}
\resizebox{\textwidth}{!}{
\begin{tabular}{b{3.5cm}<{\centering}   c c c c c c  }
    \multirow{2}{*}[-0.5em]{\makecell[c]{\vspace{0.1cm}Evaluate in \\ FLOW}} & \multicolumn{6}{c}{\texttt{Intersection}}  \\
    \cline{2-7}  \vspace{-3mm}\\ 
    & Success ($\uparrow$) & Collision ($\downarrow$) & Off Road ($\downarrow$) & Off Route ($\downarrow$) & Wrong Lane ($\downarrow$) & Efficiency ($\uparrow$)   \\
    \cline{1-7}  \vspace{-2mm}\\ 
    \rowcolor{priormethod} {RARL/FailMaker}        & 26.0  & 13.5  & 13.0  & 16.0  & 0.5  & 25.7   \\
    \rowcolor{priormethod} {VRL/IDM}            & 65.5 & 18.5 & 13.0 & \textbf{1.5} & 0.5&  42.8 \\
    \rowcolor{ourmethod} {VRL/FLOW}            & 87.5 & 6.5 & 1.5 & 0.0 & 0.0&  51.5   \\
    \rowcolor{priormethod} {VRL/CoPO}              & 76.0 & 12.0 & \textbf{2.0} & 3.0 & \textbf{0.0} &  46.5  \\
    \rowcolor{priormethod} {VRL/SocialComm}    & 79.0 & 11.0 & \textbf{2.0} & 4.5 & \textbf{0.0} & 47.9   \\
    \rowcolor{priormethod} {M-RARL/SocialComm}$^\dagger$     & \textbf{83.5} & \textbf{8.0} & \textbf{2.0} & 3.0 & 0.5& \textbf{49.7} \\
    % \rowcolor{priormethod} {M-RARL/SocialComm}$^\dagger$     & 85.5  & 9.5  & 0.0  & 0.0  & 0.0  & 50.3 \\
    \bottomrule
\end{tabular}}
\resizebox{\textwidth}{!}{
\begin{tabular}{b{3.5cm}<{\centering}   c c c c c c  }
    \multirow{2}{*}[-0.5em]{\makecell[c]{\vspace{0.1cm}Evaluate in \\ CoPO}} & \multicolumn{6}{c}{\texttt{Intersection}}  \\
    \cline{2-7}  \vspace{-3mm}\\ 
    & Success ($\uparrow$) & Collision ($\downarrow$) & Off Road ($\downarrow$) & Off Route ($\downarrow$) & Wrong Lane ($\downarrow$) & Efficiency ($\uparrow$)   \\
    \cline{1-7}  \vspace{-2mm}\\ 
    \rowcolor{priormethod} {RARL/FailMaker}        & 25.5  & \textbf{11.5}  & 15.5  & 14.5  & 0.5  & 26.0  \\
    \rowcolor{priormethod} {VRL/IDM}            & 69.5 & 20.0 & 8.0 & 1.0 & 0.5& 45.0    \\
    \rowcolor{priormethod} {VRL/FLOW}           & 75.5 & 20.0 & 1.5 & \textbf{0.0} & \textbf{0.0}&  46.1  \\
    \rowcolor{ourmethod} {VRL/CoPO}             & 81.5 & 16.0 & 1.0 & 0.0 & 0.0&  48.7  \\
    \rowcolor{priormethod} {VRL/SocialComm}    & 74.5 & 19.0 & 1.0 & 2.0 & \textbf{0.0}& 45.8   \\
    \rowcolor{priormethod} {M-RARL/SocialComm}$^\dagger$     & \textbf{79.5} & 16.5 & \textbf{0.0} & 1.0 & \textbf{0.0}&  \textbf{47.7} \\
    % \rowcolor{priormethod} {M-RARL/SocialComm}$^\dagger$     & 77.5  & 17.5  & 1.0  & 0.0  & 0.0  & 46.4  \\
    \bottomrule
\end{tabular}}
\resizebox{\textwidth}{!}{
\begin{tabular}{b{3.5cm}<{\centering}   c c c c c c  }
    \multirow{2}{*}[-0.5em]{\makecell[c]{\vspace{0.1cm}Evaluate in \\ SocialComm}} & \multicolumn{6}{c}{\texttt{Intersection}}  \\
    \cline{2-7}  \vspace{-3mm}\\ 
    & Success ($\uparrow$) & Collision ($\downarrow$) & Off Road ($\downarrow$) & Off Route ($\downarrow$) & Wrong Lane ($\downarrow$) & Efficiency ($\uparrow$)   \\
    \cline{1-7}  \vspace{-2mm}\\ 
    \rowcolor{priormethod} {RARL/FailMaker}            & 21.5  & 12.5  & 21.0  & 15.0  & 0.5  & 24.9  \\
    \rowcolor{priormethod} {VRL/IDM}            & 77.0 & \textbf{10.0} & 11.0 & 1.0 & \textbf{0.0}&  47.1  \\
    \rowcolor{priormethod} {VRL/FLOW}            & 84.0 & 13.5 & \textbf{1.0} & \textbf{0.5} & 0.5&  50.1 \\
    \rowcolor{priormethod} {VRL/CoPO}             & 81.5 & 14.5 & \textbf{1.0} & 2.0 & \textbf{0.0}&  48.8   \\
    \rowcolor{ourmethod} {VRL/SocialComm}    & 87.0 & 7.0 & 1.5 & 1.5 & 0.5&  51.9   \\
    \rowcolor{priormethod} {M-RARL/SocialComm}$^\dagger$     & \textbf{85.5} & 11.0 & \textbf{1.0} & \textbf{0.5} & \textbf{0.0}&  \textbf{50.9}   \\
    % \rowcolor{priormethod} {M-RARL/SocialComm}$^\dagger$     & 86.5  & 12.5  & 0.0  & 0.0  & 0.0  & 50.8  \\
    \bottomrule
\end{tabular}}
\resizebox{\textwidth}{!}{
\begin{tabular}{b{3.5cm}<{\centering}   c c c c c c  }
    \multirow{2}{*}[-0.5em]{\makecell[c]{\vspace{0.1cm}Evaluate in \\ SocialComm (with Adv)}} & \multicolumn{6}{c}{\texttt{Intersection}}  \\
    \cline{2-7}  \vspace{-3mm}\\ 
    & Success ($\uparrow$) & Collision ($\downarrow$) & Off Road ($\downarrow$) & Off Route ($\downarrow$) & Wrong Lane ($\downarrow$) & Efficiency ($\uparrow$)   \\
    \cline{1-7}  \vspace{-2mm}\\ 
    \rowcolor{priormethod} {RARL/FailMaker}        & 24.0  & 12.5  & 15.5  & 18.0  & 0.5  & 25.3  \\
    \rowcolor{priormethod} {VRL/IDM}            & 74.5 & 14.5 & 7.5 & 2.5 & \textbf{0.0}& 45.9  \\
    \rowcolor{priormethod} {VRL/FLOW}            & 82.5 & 15.0 & 2.0 & \textbf{0.0} & \textbf{0.0}&  49.6 \\
    \rowcolor{priormethod} {VRL/CoPO}              & 78.5 & 18.5 & \textbf{1.5} & 1.0 & \textbf{0.0}& 47.5    \\
    \rowcolor{priormethod} {VRL/SocialComm}    & \textbf{85.0} & \textbf{9.0} & 3.0 & 1.0 & 0.5& \textbf{50.8} \\
    \rowcolor{ourmethod} {M-RARL/SocialComm}$^\dagger$     & 86.0 & 10.5 & 0.5 & 1.5 & 0.0&  51.4 \\
    % \rowcolor{priormethod} {M-RARL/SocialComm}$^\dagger$   & 85.5  & 12.0  & 1.0  & 0.0  & 0.0  & 50.5    \\
    \bottomrule
\end{tabular}}

\end{table*}

\begin{table*}[htb]
\centering
\caption{{\bf {Zero-shot transfer performance in \texttt{bottleneck}.}} Each subtable stores results of different driving policies in the same traffic flow. A ``$^\dagger$" indicates the proposed method.}
\label{appendix-table:ood-performance-bottleneck}
 % default is 1.0
\resizebox{\textwidth}{!}{
\begin{tabular}{b{3.5cm}<{\centering}   c c c c c c }
    \toprule
    \multirow{2}{*}[-0.5em]{\makecell[c]{\vspace{0.1cm}Evaluate in \\ FailMaker}} & \multicolumn{6}{c}{\texttt{Bottleneck}}  \\
    \cline{2-7}  \vspace{-3mm}\\ 
    & Success ($\uparrow$) & Collision ($\downarrow$) & Off Road ($\downarrow$) & Off Route ($\downarrow$) & Wrong Lane ($\downarrow$) & Efficiency ($\uparrow$)   \\
    \cline{1-7}  \vspace{-2mm}\\ 
    \rowcolor{ourmethod} {RARL/FailMaker}                 & 38.0  & 23.0  & 38.5  & 0.5  & 0.0  & 26.1  \\
    \rowcolor{priormethod} {VRL/IDM}                & \textbf{20.5}  & \textbf{59.0}  & 26.0  & \textbf{0.0}  & \textbf{0.0}  & \textbf{34.5}  \\
    \rowcolor{priormethod} {VRL/FLOW}               & 4.5  & 94.0  & 3.0  & \textbf{0.0}  & \textbf{0.0}  & 24.2 \\
    \rowcolor{priormethod} {VRL/CoPO}               & 6.5  & 88.5  & 6.5  & \textbf{0.0}  & \textbf{0.0}  & 27.5  \\
    \rowcolor{priormethod} {VRL/SocialComm}     & 2.5  & 87.5  & 13.5  & \textbf{0.0}  & \textbf{0.0}  & 24.3  \\
    \rowcolor{priormethod} {M-RARL/SocialComm}$^\dagger$        & 4.5  & 94.0  & \textbf{2.0}  & \textbf{0.0}  & \textbf{0.0}  & 24.1 \\
    % \rowcolor{priormethod} {M-RARL/SocialComm}$^\dagger$        & 7.0  & 86.0  & 9.0  & 0.0  & 0.0  & 26.2 \\
    \bottomrule
\end{tabular}}
\resizebox{\textwidth}{!}{
\begin{tabular}{b{3.5cm}<{\centering}   c c c c c c }
    \multirow{2}{*}[-0.5em]{\makecell[c]{\vspace{0.1cm}Evaluate in \\ IDM}} & \multicolumn{6}{c}{\texttt{Bottleneck}}  \\
    \cline{2-7}  \vspace{-3mm}\\ 
    & Success ($\uparrow$) & Collision ($\downarrow$) & Off Road ($\downarrow$) & Off Route ($\downarrow$) & Wrong Lane ($\downarrow$) & Efficiency ($\uparrow$)   \\
    \cline{1-7}  \vspace{-2mm}\\ 
    \rowcolor{priormethod} {RARL/FailMaker}                  & 50.0  & \textbf{10.0}  & 37.5  & 3.0  & \textbf{0.0}  & 33.9  \\
    \rowcolor{ourmethod} {VRL/IDM}               & 91.5 & 6.0 & 2.5 & 0.0 & 0.0 &  72.8  \\
    \rowcolor{priormethod} {VRL/FLOW}               & 53.0 & 25.5 & 19.5 & 2.5 & \textbf{0.0} &  51.7  \\
    \rowcolor{priormethod} {VRL/CoPO}               & 64.5 & 24.0 & 10.5 & 2.5 & \textbf{0.0} &   \textbf{59.6} \\
    \rowcolor{priormethod} {VRL/SocialComm}     & 67.0 & 20.5 & 12.5 & \textbf{0.0} & \textbf{0.0} &  55.8 \\
    \rowcolor{priormethod} {M-RARL/SocialComm}$^\dagger$        & \textbf{74.5} & 21.0 & \textbf{5.5} & \textbf{0.0} & \textbf{0.0} & 57.6 \\
    % \rowcolor{priormethod} {M-RARL/SocialComm}$^\dagger$        & 75.0  & 19.0  & 6.0  & 0.0  & 0.0  & 58.8 \\
    \bottomrule
\end{tabular}}
\resizebox{\textwidth}{!}{
\begin{tabular}{b{3.5cm}<{\centering}   c c c c c c }
    \multirow{2}{*}[-0.5em]{\makecell[c]{\vspace{0.1cm}Evaluate in \\ FLOW}} & \multicolumn{6}{c}{\texttt{Bottleneck}}  \\
    \cline{2-7}  \vspace{-3mm}\\ 
    & Success ($\uparrow$) & Collision ($\downarrow$) & Off Road ($\downarrow$) & Off Route ($\downarrow$) & Wrong Lane ($\downarrow$) & Efficiency ($\uparrow$)   \\
    \cline{1-7}  \vspace{-2mm}\\ 
    \rowcolor{priormethod} {RARL/FailMaker}                  & 42.0  & \textbf{18.5}  & 39.5  & \textbf{0.0}  & \textbf{0.0}  & 25.6  \\
    \rowcolor{priormethod} {VRL/IDM}                & 51.0 & 24.0 & 26.5 & 0.5 & \textbf{0.0}  &  54.8 \\
    \rowcolor{ourmethod} {VRL/FLOW}              & 79.0 & 18.5 & 2.0 & 0.5 & 0.0 &  76.1  \\
    \rowcolor{priormethod} {VRL/CoPO}               & 60.5 & 27.5 & 12.5 & \textbf{0.0} & \textbf{0.0} &  65.5  \\
    \rowcolor{priormethod} {VRL/SocialComm}     & 72.5 & 24.0 & 4.5 & \textbf{0.0} & \textbf{0.0}  &  \textbf{68.7} \\
    \rowcolor{priormethod} {M-RARL/SocialComm}$^\dagger$        & \textbf{73.0} & 25.5 & \textbf{2.0} & \textbf{0.0} & \textbf{0.0} &  68.4  \\
    % \rowcolor{priormethod} {M-RARL/SocialComm}$^\dagger$        & 79.0  & 13.5  & 8.0  & 0.0  & 0.0  & 73.1  \\
    \bottomrule
\end{tabular}}
\resizebox{\textwidth}{!}{
\begin{tabular}{b{3.5cm}<{\centering}   c c c c c c }
    \multirow{2}{*}[-0.5em]{\makecell[c]{\vspace{0.1cm}Evaluate in \\ CoPO}} & \multicolumn{6}{c}{\texttt{Bottleneck}}  \\
    \cline{2-7}  \vspace{-3mm}\\ 
    & Success ($\uparrow$) & Collision ($\downarrow$) & Off Road ($\downarrow$) & Off Route ($\downarrow$) & Wrong Lane ($\downarrow$) & Efficiency ($\uparrow$)   \\
    \cline{1-7}  \vspace{-2mm}\\ 
    \rowcolor{priormethod} {RARL/FailMaker}                  & 51.0  & 11.0  & 34.5  & 3.5  & \textbf{0.0}  & 35.1  \\
    \rowcolor{priormethod} {VRL/IDM}                & 48.5 & 16.5 & 33.0 & 2.0 & \textbf{0.0}  &  57.2 \\
    \rowcolor{priormethod} {VRL/FLOW}               & 61.0 & \textbf{6.5} & 33.0 & \textbf{0.0} & \textbf{0.0}  &   64.6\\
    \rowcolor{ourmethod} {VRL/CoPO}              & 89.0 & 9.0 & 1.5 & 0.5 & 0.0 &  81.8  \\
    \rowcolor{priormethod} {VRL/SocialComm}     & 65.0 & 30.5 & 5.5 & \textbf{0.0} & \textbf{0.0}  &  67.2 \\
    \rowcolor{priormethod} {M-RARL/SocialComm}$^\dagger$        & \textbf{74.0} & 25.5 & \textbf{0.5} & \textbf{0.0} & \textbf{0.0}  &  \textbf{71.0} \\
    % \rowcolor{priormethod} {M-RARL/SocialComm}$^\dagger$        & 83.0  & 8.0  & 10.0  & 0.0  & 0.0  & 74.6 \\
    \bottomrule
\end{tabular}}
\resizebox{\textwidth}{!}{
\begin{tabular}{b{3.5cm}<{\centering}   c c c c c c }
    \multirow{2}{*}[-0.5em]{\makecell[c]{\vspace{0.1cm}Evaluate in \\ SocialComm}} & \multicolumn{6}{c}{\texttt{Bottleneck}}  \\
    \cline{2-7}  \vspace{-3mm}\\ 
    & Success ($\uparrow$) & Collision ($\downarrow$) & Off Road ($\downarrow$) & Off Route ($\downarrow$) & Wrong Lane ($\downarrow$) & Efficiency ($\uparrow$)   \\
    \cline{1-7}  \vspace{-2mm}\\ 
    \rowcolor{priormethod} {RARL/FailMaker}                  & 36.0 & 23.5 & 42.0 & 0.5 & \textbf{0.0} & 26.6 \\
    \rowcolor{priormethod} {VRL/IDM}                & 52.5 & 26.0 & 21.0 & 0.5 & \textbf{0.0} & 58.3  \\
    \rowcolor{priormethod} {VRL/FLOW}               & 75.5 & 19.5 & 4.5 & 0.5 & \textbf{0.0} &  74.6 \\
    \rowcolor{priormethod} {VRL/CoPO}               & 71.5 & 13.5 & 15.5 & 1.0 & \textbf{0.0} & 70.9  \\
    \rowcolor{ourmethod} {VRL/SocialComm}    & 91.0 & 4.0 & 5.0 & 0.0 & 0.0 & 81.3  \\
    \rowcolor{priormethod} {M-RARL/SocialComm}$^\dagger$        & \textbf{89.5} & \textbf{8.5} & \textbf{2.0} & \textbf{0.0} & \textbf{0.0} &  \textbf{79.6} \\
    % \rowcolor{priormethod} {M-RARL/SocialComm}$^\dagger$        & 85.0  & 9.5  & 5.5  & 0.0  & 0.0  & 76.9 \\
    \bottomrule
\end{tabular}}
\resizebox{\textwidth}{!}{
\begin{tabular}{b{3.5cm}<{\centering}   c c c c c c }
    \multirow{2}{*}[-0.5em]{\makecell[c]{\vspace{0.1cm}Evaluate in \\ SocialComm (with Adv)}} & \multicolumn{6}{c}{\texttt{Bottleneck}}  \\
    \cline{2-7}  \vspace{-3mm}\\ 
    & Success ($\uparrow$) & Collision ($\downarrow$) & Off Road ($\downarrow$) & Off Route ($\downarrow$) & Wrong Lane ($\downarrow$) & Efficiency ($\uparrow$)   \\
    \cline{1-7}  \vspace{-2mm}\\ 
    \rowcolor{priormethod} {RARL/FailMaker}                  & 36.5  & 19.0  & 43.5  & 1.0  & \textbf{0.0}  & 27.7  \\
    \rowcolor{priormethod} {VRL/IDM}                & 50.5 & 27.0 & 22.0 & 0.5 & \textbf{0.0}  &   57.0 \\
    \rowcolor{priormethod} {VRL/FLOW}               & 73.5 & 24.0 & \textbf{2.0} & 0.5 & \textbf{0.0}  &   73.8\\
    \rowcolor{priormethod} {VRL/CoPO}               & 69.5 & 11.0 & 19.0 & 1.0 & \textbf{0.0}  &  69.9 \\
    \rowcolor{priormethod} {VRL/SocialComm}     & \textbf{85.0} & \textbf{7.0} & 8.0 & \textbf{0.0} & \textbf{0.0}  &  \textbf{78.3} \\
    \rowcolor{ourmethod} {M-RARL/SocialComm}$^\dagger$       & 88.5 & 11.5 & 0.0 & 0.0 & 0.0  &  79.8 \\
    % \rowcolor{ourmethod} {M-RARL/SocialComm}$^\dagger$       & 88.0  & 8.5  & 3.5  & 0.0  & 0.0  & 78.7 \\
    \bottomrule
\end{tabular}}

\end{table*}

\begin{table*}[htb]
\centering
\caption{{\bf {Zero-shot transfer performance in \texttt{merge}.}} Each subtable stores results of different driving policies in the same traffic flow. A ``$^\dagger$" indicates the proposed method.}
\label{appendix-table:ood-performance-merge}
 % default is 1.0
\resizebox{\textwidth}{!}{
\begin{tabular}{b{3.5cm}<{\centering}   c c c c c c  }
    \toprule
    \multirow{2}{*}[-0.5em]{\makecell[c]{\vspace{0.1cm}Evaluate in \\ FailMaker}} & \multicolumn{6}{c}{\texttt{Merge}}  \\
    \cline{2-7}  \vspace{-3mm}\\ 
    & Success ($\uparrow$) & Collision ($\downarrow$) & Off Road ($\downarrow$) & Off Route ($\downarrow$) & Wrong Lane ($\downarrow$) & Efficiency ($\uparrow$)   \\
    \cline{1-7}  \vspace{-2mm}\\ 
    \rowcolor{ourmethod} {RARL/FailMaker}        & 19.5  & 37.5  & 39.5  & 6.5  & 0.0  & 21.6     \\
    \rowcolor{priormethod} {VRL/IDM}            & 9.0  & \textbf{74.5}  & 18.0  & \textbf{0.0}  & \textbf{0.0}  & 15.1  \\
    \rowcolor{priormethod} {VRL/FLOW}           & 9.0  & 81.0  & 11.5  & \textbf{0.0}  & \textbf{0.0}  & 17.5  \\
    \rowcolor{priormethod} {VRL/CoPO}            & 10.0  & 83.5  & 10.0  & \textbf{0.0}  & \textbf{0.0}  & \textbf{19.2}   \\
    \rowcolor{priormethod} {VRL/SocialComm}    & 8.5  & 88.0  & \textbf{4.0}  & \textbf{0.0}  & \textbf{0.0}  & 16.8   \\
    \rowcolor{priormethod} {M-RARL/SocialComm}$^\dagger$     & \textbf{12.0}  & 78.5  & 11.0  & \textbf{0.0}  & \textbf{0.0}  & 18.5   \\
    % \rowcolor{priormethod} {M-RARL/SocialComm}$^\dagger$     & 13.0  & 80.0  & 10.0  & 0.0  & 0.0  & 19.2   \\
    \bottomrule
\end{tabular}}
\resizebox{\textwidth}{!}{
\begin{tabular}{b{3.5cm}<{\centering}   c c c c c c  }
    \multirow{2}{*}[-0.5em]{\makecell[c]{\vspace{0.1cm}Evaluate in \\ IDM}} & \multicolumn{6}{c}{\texttt{Merge}}  \\
    \cline{2-7}  \vspace{-3mm}\\ 
    & Success ($\uparrow$) & Collision ($\downarrow$) & Off Road ($\downarrow$) & Off Route ($\downarrow$) & Wrong Lane ($\downarrow$) & Efficiency ($\uparrow$)   \\
    \cline{1-7}  \vspace{-2mm}\\ 
    \rowcolor{priormethod} {RARL/FailMaker}                & 66.5  & \textbf{5.0}  & 14.5  & 14.0  & \textbf{0.0}  & 45.9    \\
    \rowcolor{ourmethod} {VRL/IDM}            & 92.0  & 6.0  & 2.0  & 0.0  & 0.0  & 62.3  \\
    \rowcolor{priormethod} {VRL/FLOW}           & 41.5  & 55.5  & 7.5  & 0.5  & \textbf{0.0}  & 29.1  \\
    \rowcolor{priormethod} {VRL/CoPO}            & 54.5  & 19.0  & 22.5  & 9.0  & \textbf{0.0}  & 38.0  \\
    \rowcolor{priormethod} {VRL/SocialComm}    & 67.5  & 18.5  & 14.5  & \textbf{0.0}  & \textbf{0.0}  & 43.6 \\
    \rowcolor{priormethod} {M-RARL/SocialComm}$^\dagger$     & \textbf{85.0}  & 15.0  & \textbf{0.0}  & \textbf{0.0}  & \textbf{0.0}  & \textbf{53.2}  \\
    % \rowcolor{priormethod} {M-RARL/SocialComm}$^\dagger$     & 89.0  & 11.0  & 0.0  & 0.0  & 0.0  & 57.8  \\
    \bottomrule
\end{tabular}}
\resizebox{\textwidth}{!}{
\begin{tabular}{b{3.5cm}<{\centering}   c c c c c c  }
    \multirow{2}{*}[-0.5em]{\makecell[c]{\vspace{0.1cm}Evaluate in \\ FLOW}} & \multicolumn{6}{c}{\texttt{Merge}}  \\
    \cline{2-7}  \vspace{-3mm}\\ 
    & Success ($\uparrow$) & Collision ($\downarrow$) & Off Road ($\downarrow$) & Off Route ($\downarrow$) & Wrong Lane ($\downarrow$) & Efficiency ($\uparrow$)   \\
    \cline{1-7}  \vspace{-2mm}\\ 
    \rowcolor{priormethod} {RARL/FailMaker}        & 17.0  & 40.5  & 33.5  & 9.5  & \textbf{0.0}  & 24.2   \\
    \rowcolor{priormethod} {VRL/IDM}            & 35.0  & 38.0  & 27.5  & \textbf{0.0}  & \textbf{0.0}  & 40.5 \\
    \rowcolor{ourmethod} {VRL/FLOW}            & 69.5  & 25.0  & 5.5  & 0.0  & 0.0  & 56.0   \\
    \rowcolor{priormethod} {VRL/CoPO}              & 52.0  & 35.0  & 12.0  & 1.0  & \textbf{0.0}  & 48.2  \\
    \rowcolor{priormethod} {VRL/SocialComm}    & 62.5  & 33.5  & \textbf{4.0}  & \textbf{0.0}  & \textbf{0.0}  & 54.5   \\
    \rowcolor{priormethod} {M-RARL/SocialComm}$^\dagger$     & \textbf{67.5}  & \textbf{21.5}  & 11.0  & \textbf{0.0}  & \textbf{0.0}  & \textbf{56.0} \\
    % \rowcolor{priormethod} {M-RARL/SocialComm}$^\dagger$     & 68.0  & 24.5  & 8.0  & 0.0  & 0.0  & 55.8 \\
    \bottomrule
\end{tabular}}
\resizebox{\textwidth}{!}{
\begin{tabular}{b{3.5cm}<{\centering}   c c c c c c  }
    \multirow{2}{*}[-0.5em]{\makecell[c]{\vspace{0.1cm}Evaluate in \\ CoPO}} & \multicolumn{6}{c}{\texttt{Merge}}  \\
    \cline{2-7}  \vspace{-3mm}\\ 
    & Success ($\uparrow$) & Collision ($\downarrow$) & Off Road ($\downarrow$) & Off Route ($\downarrow$) & Wrong Lane ($\downarrow$) & Efficiency ($\uparrow$)   \\
    \cline{1-7}  \vspace{-2mm}\\ 
    \rowcolor{priormethod} {RARL/FailMaker}        & 17.0  & 39.0  & 34.0  & 10.0  & \textbf{0.0}  & 23.5  \\
    \rowcolor{priormethod} {VRL/IDM}            & 36.5  & 44.5  & 19.0  & \textbf{0.0}  & \textbf{0.0}  & 40.0    \\
    \rowcolor{priormethod} {VRL/FLOW}           & 50.0  & 44.0  & 5.5  & 0.5  & \textbf{0.0}  & 46.6  \\
    \rowcolor{ourmethod} {VRL/CoPO}             & 70.5  & 24.5  & 5.0  & 0.0  & 0.0  & 55.4  \\
    \rowcolor{priormethod} {VRL/SocialComm}    & 57.0  & \textbf{37.5}  & 5.5  & \textbf{0.0}  & \textbf{0.0}  & 49.9   \\
    \rowcolor{priormethod} {M-RARL/SocialComm}$^\dagger$     & \textbf{59.5}  & 40.0  & \textbf{0.5}  & \textbf{0.0}  & \textbf{0.0}  & \textbf{52.0} \\
    % \rowcolor{priormethod} {M-RARL/SocialComm}$^\dagger$     & 66.5  & 26.5  & 7.0  & 0.0  & 0.0  & 52.9 \\
    \bottomrule
\end{tabular}}
\resizebox{\textwidth}{!}{
\begin{tabular}{b{3.5cm}<{\centering}   c c c c c c  }
    \multirow{2}{*}[-0.5em]{\makecell[c]{\vspace{0.1cm}Evaluate in \\ SocialComm}} & \multicolumn{6}{c}{\texttt{Merge}}  \\
    \cline{2-7}  \vspace{-3mm}\\ 
    & Success ($\uparrow$) & Collision ($\downarrow$) & Off Road ($\downarrow$) & Off Route ($\downarrow$) & Wrong Lane ($\downarrow$) & Efficiency ($\uparrow$)   \\
    \cline{1-7}  \vspace{-2mm}\\ 
    \rowcolor{priormethod} {RARL/FailMaker}            & 18.5  & 29.0  & 47.5  & 6.5  & \textbf{0.0}  & 27.6  \\
    \rowcolor{priormethod} {VRL/IDM}            & 65.0  & 16.0  & 19.0  & \textbf{0.0}  & \textbf{0.0}  & 51.3  \\
    \rowcolor{priormethod} {VRL/FLOW}            & 71.5  & 21.0  & 7.5  & \textbf{0.0}  & \textbf{0.0}  & 55.0\\
    \rowcolor{priormethod} {VRL/CoPO}             & 70.0  & 24.5  & 5.5  & 0.5  & \textbf{0.0}  & 55.1   \\
    \rowcolor{ourmethod} {VRL/SocialComm}    & 84.5  & 14.0  & 1.5  & 0.0  & 0.0  & 60.7   \\
    \rowcolor{priormethod} {M-RARL/SocialComm}$^\dagger$     & \textbf{83.5}  & \textbf{12.5}  & \textbf{3.5}  & 0.5  & \textbf{0.0}  & \textbf{61.2}   \\
    % \rowcolor{priormethod} {M-RARL/SocialComm}$^\dagger$     & 83.0  & 16.5  & 0.5  & 0.0  & 0.0  & 60.2   \\
    \bottomrule
\end{tabular}}
\resizebox{\textwidth}{!}{
\begin{tabular}{b{3.5cm}<{\centering}   c c c c c c  }
    \multirow{2}{*}[-0.5em]{\makecell[c]{\vspace{0.1cm}Evaluate in \\ SocialComm (with Adv)}} & \multicolumn{6}{c}{\texttt{Merge}}  \\
    \cline{2-7}  \vspace{-3mm}\\ 
    & Success ($\uparrow$) & Collision ($\downarrow$) & Off Road ($\downarrow$) & Off Route ($\downarrow$) & Wrong Lane ($\downarrow$) & Efficiency ($\uparrow$)   \\
    \cline{1-7}  \vspace{-2mm}\\ 
    \rowcolor{priormethod} {RARL/FailMaker}                 & 18.5  & 25.0  & 50.5  & 7.0  & \textbf{0.0}  & 27.2  \\
    \rowcolor{priormethod} {VRL/IDM}            &  62.5  & 20.0  & 17.5  & \textbf{0.0}  & \textbf{0.0}  & 50.7 \\
    \rowcolor{priormethod} {VRL/FLOW}            & 69.5  & 22.5  & 8.0  & \textbf{0.0}  & \textbf{0.0}  & 54.1 \\
    \rowcolor{priormethod} {VRL/CoPO}              & 66.0  & 23.5  & 10.5  & 0.5  & \textbf{0.0}  & 53.4    \\
    \rowcolor{priormethod} {VRL/SocialComm}    & \textbf{80.0}  & \textbf{19.5}  & \textbf{0.5}  & \textbf{0.0}  & \textbf{0.0}  & \textbf{59.2} \\
    \rowcolor{ourmethod} {M-RARL/SocialComm}$^\dagger$     & 85.0  & 13.5  & 1.5  & 0.0  & 0.0  & 61.3 \\
    \bottomrule
\end{tabular}}

\end{table*}

\begin{table*}[htb]
\centering
\caption{{\bf {Zero-shot transfer performance in \texttt{roundabout}.}} Each subtable stores results of different driving policies in the same traffic flow. A ``$^\dagger$" indicates the proposed method.}
\label{appendix-table:ood-performance-roundabout}
 % default is 1.0
\resizebox{\textwidth}{!}{
\begin{tabular}{b{3.5cm}<{\centering}   c c c c c c  }
    \toprule
    \multirow{2}{*}[-0.5em]{\makecell[c]{\vspace{0.1cm}Evaluate in \\ FailMaker}} & \multicolumn{6}{c}{\texttt{Roundabout}}  \\
    \cline{2-7}  \vspace{-3mm}\\ 
    & Success ($\uparrow$) & Collision ($\downarrow$) & Off Road ($\downarrow$) & Off Route ($\downarrow$) & Wrong Lane ($\downarrow$) & Efficiency ($\uparrow$)   \\
    \cline{1-7}  \vspace{-2mm}\\ 
    \rowcolor{ourmethod} {RARL/FailMaker}              & 29.5  & 17.0  & 51.5  & 5.0  & \textbf{0.0}  & 14.5     \\
    \rowcolor{priormethod} {VRL/IDM}            & 19.5  & 64.0  & 20.5  & \textbf{0.0}  & 0.5  & 20.2   \\
    \rowcolor{priormethod} {VRL/FLOW}           & \textbf{29.5}  & \textbf{57.5}  & 14.0  & \textbf{0.0}  & \textbf{0.0}  & \textbf{25.0}  \\
    \rowcolor{priormethod} {VRL/CoPO}            & 21.0  & 70.5  & \textbf{10.0}  & \textbf{0.0}  & 0.5  & 22.7   \\
    \rowcolor{priormethod} {VRL/SocialComm}    & 17.0  & 63.0  & 24.5  & \textbf{0.0}  & \textbf{0.0}  & 19.9   \\
    \rowcolor{priormethod} {M-RARL/SocialComm}$^\dagger$     & 18.5  & \textbf{57.5}  & 25.5  & \textbf{0.0}  & \textbf{0.0}  & 20.5   \\
    % \rowcolor{priormethod} {M-RARL/SocialComm}$^\dagger$     & 31.0  & 58.0  & 13.0  & 0.0  & 0.0  & 26.0   \\
    \bottomrule
\end{tabular}}
\resizebox{\textwidth}{!}{
\begin{tabular}{b{3.5cm}<{\centering}   c c c c c c  }
    \multirow{2}{*}[-0.5em]{\makecell[c]{\vspace{0.1cm}Evaluate in \\ IDM}} & \multicolumn{6}{c}{\texttt{Roundabout}}  \\
    \cline{2-7}  \vspace{-3mm}\\ 
    & Success ($\uparrow$) & Collision ($\downarrow$) & Off Road ($\downarrow$) & Off Route ($\downarrow$) & Wrong Lane ($\downarrow$) & Efficiency ($\uparrow$)   \\
    \cline{1-7}  \vspace{-2mm}\\ 
    \rowcolor{priormethod} {RARL/FailMaker}                & 32.5  & \textbf{16.0}  & 55.5  & 6.0  & 0.5  & 19.7    \\
    \rowcolor{ourmethod} {VRL/IDM}            & 83.0  & 9.0  & 5.5  & 0.0  & 2.5  & 38.7  \\
    \rowcolor{priormethod} {VRL/FLOW}           & 44.5  & 51.5  & \textbf{4.0}  & 1.0  & \textbf{0.0}  & 23.8  \\
    \rowcolor{priormethod} {VRL/CoPO}            & 59.0  & 33.0  & 9.5  & \textbf{0.0}  & \textbf{0.0}  & 31.5  \\
    \rowcolor{priormethod} {VRL/SocialComm}    & 40.5  & 30.5  & 31.0  & 0.5  & 1.0  & 21.1 \\
    \rowcolor{priormethod} {M-RARL/SocialComm}$^\dagger$     & \textbf{63.0}  & 18.5  & 17.0  & \textbf{0.0}  & 1.5  & \textbf{32.3}  \\
    % \rowcolor{priormethod} {M-RARL/SocialComm}$^\dagger$     & 73.0  & 22.0  & 5.0  & 0.0  & 0.0  & 35.3   \\
    \bottomrule
\end{tabular}}
\resizebox{\textwidth}{!}{
\begin{tabular}{b{3.5cm}<{\centering}   c c c c c c  }
    \multirow{2}{*}[-0.5em]{\makecell[c]{\vspace{0.1cm}Evaluate in \\ FLOW}} & \multicolumn{6}{c}{\texttt{Roundabout}}  \\
    \cline{2-7}  \vspace{-3mm}\\ 
    & Success ($\uparrow$) & Collision ($\downarrow$) & Off Road ($\downarrow$) & Off Route ($\downarrow$) & Wrong Lane ($\downarrow$) & Efficiency ($\uparrow$)   \\
    \cline{1-7}  \vspace{-2mm}\\ 
    \rowcolor{priormethod} {RARL/FailMaker}        & 30.5  & \textbf{24.0}  & 46.0  & 5.0  & 0.5  & 17.7  \\
    \rowcolor{priormethod} {VRL/IDM}            & 54.0  & 27.0  & 18.5  & \textbf{0.0}  & 0.5  & 32.7 \\
    \rowcolor{ourmethod} {VRL/FLOW}            & 84.0  & 11.5  & 4.5  & 0.0  & 0.0  & 42.7   \\
    \rowcolor{priormethod} {VRL/CoPO}              & 61.5  & 29.5  & 9.0  & \textbf{0.0}  & \textbf{0.0}  & 38.4  \\
    \rowcolor{priormethod} {VRL/SocialComm}    & 66.5  & 25.5  & 9.5  & \textbf{0.0}  & \textbf{0.0}  & 38.6   \\
    \rowcolor{priormethod} {M-RARL/SocialComm}$^\dagger$     & \textbf{70.5}  & 26.5  & \textbf{2.5}  & \textbf{0.0}  & 0.5  & \textbf{40.1} \\
    % \rowcolor{priormethod} {M-RARL/SocialComm}$^\dagger$     & 79.5  & 17.0  & 3.5  & 0.0  & 0.0  & 41.6 \\
    \bottomrule
\end{tabular}}
\resizebox{\textwidth}{!}{
\begin{tabular}{b{3.5cm}<{\centering}   c c c c c c  }
    \multirow{2}{*}[-0.5em]{\makecell[c]{\vspace{0.1cm}Evaluate in \\ CoPO}} & \multicolumn{6}{c}{\texttt{Roundabout}}  \\
    \cline{2-7}  \vspace{-3mm}\\ 
    & Success ($\uparrow$) & Collision ($\downarrow$) & Off Road ($\downarrow$) & Off Route ($\downarrow$) & Wrong Lane ($\downarrow$) & Efficiency ($\uparrow$)   \\
    \cline{1-7}  \vspace{-2mm}\\ 
    \rowcolor{priormethod} {RARL/FailMaker}             & 32.0  & 25.0  & 46.5  & 4.5  & \textbf{0.5}  & 17.2  \\
    \rowcolor{priormethod} {VRL/IDM}            & 55.5  & 18.5  & 23.0  & 0.5  & 2.5  & 32.4    \\
    \rowcolor{priormethod} {VRL/FLOW}           & 62.0  & \textbf{12.0}  & 24.0  & \textbf{0.0}  & 2.0  & 35.7  \\
    \rowcolor{ourmethod} {VRL/CoPO}             & 86.5  & 12.0  & 1.5  & 0.0  & 0.0  & 41.8  \\
    \rowcolor{priormethod} {VRL/SocialComm}    & 70.0  & 26.5  & \textbf{3.5}  & \textbf{0.0}  & \textbf{0.5}  & 38.8   \\
    \rowcolor{priormethod} {M-RARL/SocialComm}$^\dagger$     & \textbf{76.5}  & 17.5  & 5.5  & \textbf{0.0}  & \textbf{0.5}  & \textbf{39.9} \\
    % \rowcolor{priormethod} {M-RARL/SocialComm}$^\dagger$     & 86.0  & 11.0  & 3.0  & 0.0  & 0.0  & 42.3 \\
    \bottomrule
\end{tabular}}
\resizebox{\textwidth}{!}{
\begin{tabular}{b{3.5cm}<{\centering}   c c c c c c  }
    \multirow{2}{*}[-0.5em]{\makecell[c]{\vspace{0.1cm}Evaluate in \\ SocialComm}} & \multicolumn{6}{c}{\texttt{Roundabout}}  \\
    \cline{2-7}  \vspace{-3mm}\\ 
    & Success ($\uparrow$) & Collision ($\downarrow$) & Off Road ($\downarrow$) & Off Route ($\downarrow$) & Wrong Lane ($\downarrow$) & Efficiency ($\uparrow$)   \\
    \cline{1-7}  \vspace{-2mm}\\ 
    \rowcolor{priormethod} {RARL/FailMaker}            & 30.0  & 16.5  & 54.5  & 5.0  & \textbf{0.0}  & 17.7  \\
    \rowcolor{priormethod} {VRL/IDM}            & 75.5  & \textbf{9.5}  & 13.0  & \textbf{0.0}  & 2.0  & 38.0  \\
    \rowcolor{priormethod} {VRL/FLOW}            & 74.0  & 12.0  & 14.0  & \textbf{0.0}  & \textbf{0.0}  & 39.7  \\
    \rowcolor{priormethod} {VRL/CoPO}             & 82.0  & 13.5  & \textbf{1.5}  & 1.5  & 2.5  & 42.4   \\
    \rowcolor{ourmethod} {VRL/SocialComm}    & 87.5  & 9.0  & 3.5  & 0.0  & 0.0  & 43.2   \\
    \rowcolor{priormethod} {M-RARL/SocialComm}$^\dagger$     & \textbf{86.0}  & 12.0  & 2.0  & \textbf{0.0}  & \textbf{0.0}  & \textbf{42.8}   \\
    % \rowcolor{priormethod} {M-RARL/SocialComm}$^\dagger$     & 86.0  & 11.5  & 2.5  & 0.0  & 0.0  & 43.2   \\
    \bottomrule
\end{tabular}}
\resizebox{\textwidth}{!}{
\begin{tabular}{b{3.5cm}<{\centering}   c c c c c c  }
    \multirow{2}{*}[-0.5em]{\makecell[c]{\vspace{0.1cm}Evaluate in \\ SocialComm (with Adv)}} & \multicolumn{6}{c}{\texttt{Roundabout}}  \\
    \cline{2-7}  \vspace{-3mm}\\ 
    & Success ($\uparrow$) & Collision ($\downarrow$) & Off Road ($\downarrow$) & Off Route ($\downarrow$) & Wrong Lane ($\downarrow$) & Efficiency ($\uparrow$)   \\
    \cline{1-7}  \vspace{-2mm}\\ 
    \rowcolor{priormethod} {RARL/FailMaker}                  & 31.0  & 15.5  & 56.0  & 4.5  & 0.5  & 18.2  \\
    \rowcolor{priormethod} {VRL/IDM}            & 72.5  & 13.0  & 13.0  & \textbf{0.0}  & 1.5  & 37.8 \\
    \rowcolor{priormethod} {VRL/FLOW}            & 71.5  & 16.5  & 13.5  & \textbf{0.0}  & \textbf{0.0}  & 39.5 \\
    \rowcolor{priormethod} {VRL/CoPO}              & 80.5  & 17.5  & \textbf{1.5}  & 1.0  & \textbf{0.0}  & 42.2    \\
    \rowcolor{priormethod} {VRL/SocialComm}    & \textbf{84.5}  & \textbf{11.5}  & 5.0  & \textbf{0.0}  & \textbf{0.0}  & \textbf{42.3} \\
    \rowcolor{ourmethod} {M-RARL/SocialComm}$^\dagger$     & 87.0  & 10.5  & 2.0  & 0.0  & 0.5  & 42.9 \\
    \bottomrule
\end{tabular}}

\end{table*}

% \begin{figure*}[ht]
%     \begin{center}
%     \includegraphics[width=1.0\textwidth]{image/empty_scenario_zone.pdf}
%     %%% trim={<left> <lower> <right> <upper>}
%     \end{center}
% \caption{{\color{blue} {\bf{The initial poses (makred as black arrows) and interaction zone (marked as gray rectangles) of each scenario.}}}}
% \label{figure:flow-zone}
% \end{figure*}

% \begin{figure*}[ht]
%     \begin{center}
%     \includegraphics[width=1.0\textwidth]{image/train_curve_isac.pdf}
%     %%% trim={<left> <lower> <right> <upper>}
%     \end{center}
% \vspace{-0.3cm}
% \caption{{\color{blue} {\bf{Training success rates of CoPO and SocialComm (Ours).}}}}
% \vspace{-0.3cm}
% \label{figure:train-curve}
% \end{figure*}
